# Supplementary material for: Fermionic tensor network methods
Source: arXiv:2404.14611 source file (2024-11-21)

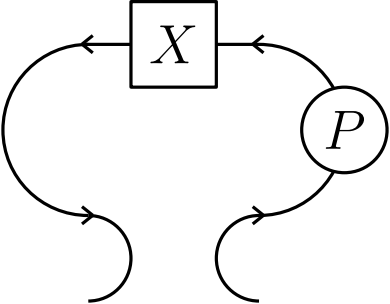

$\chi$

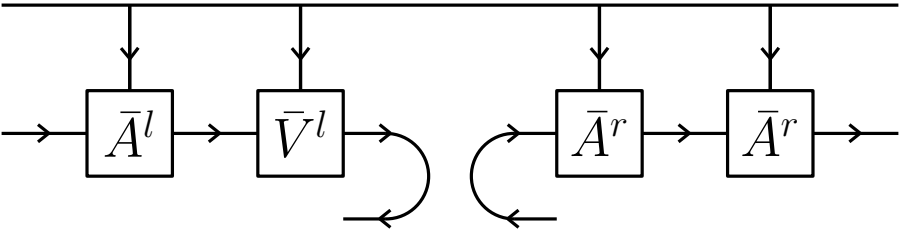

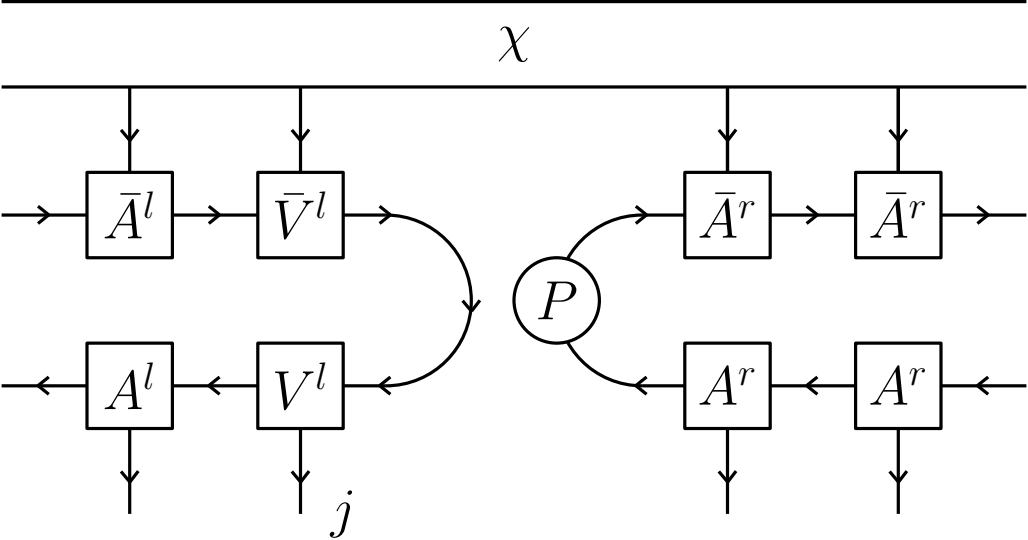

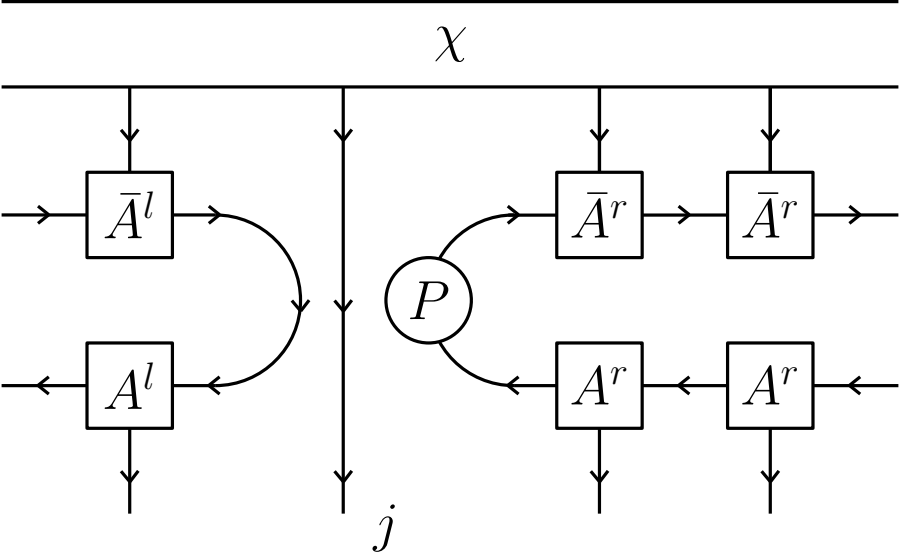

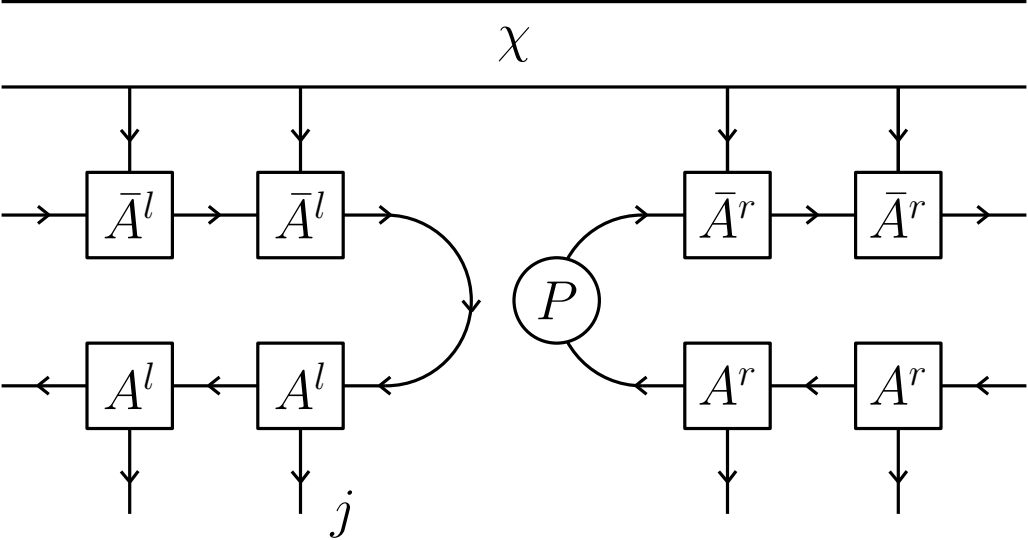

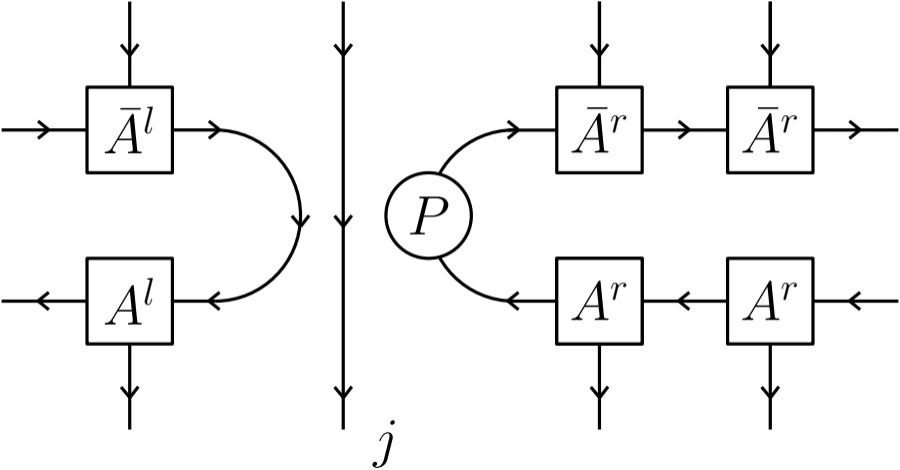

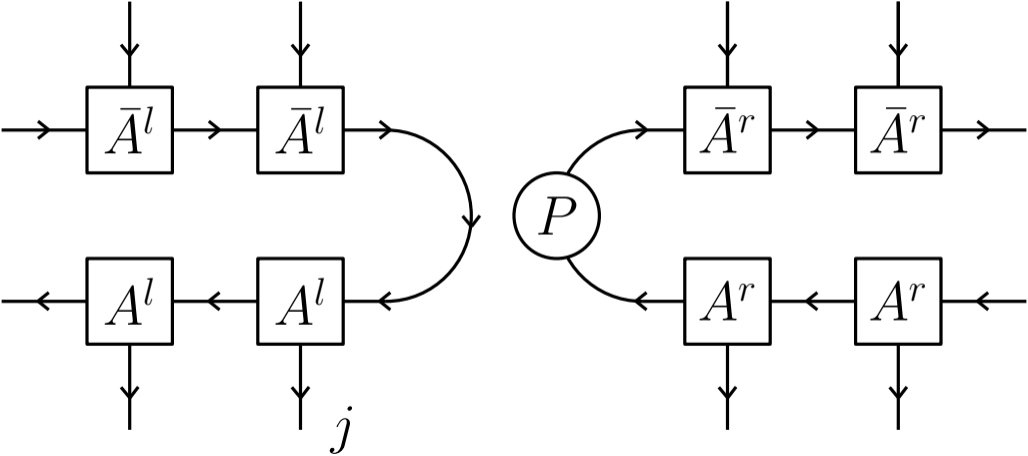

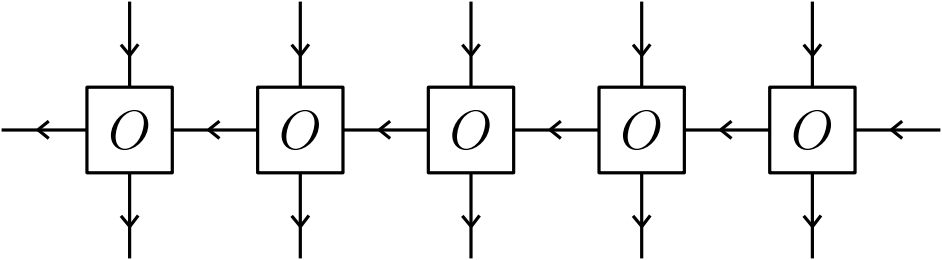

$\Psi$

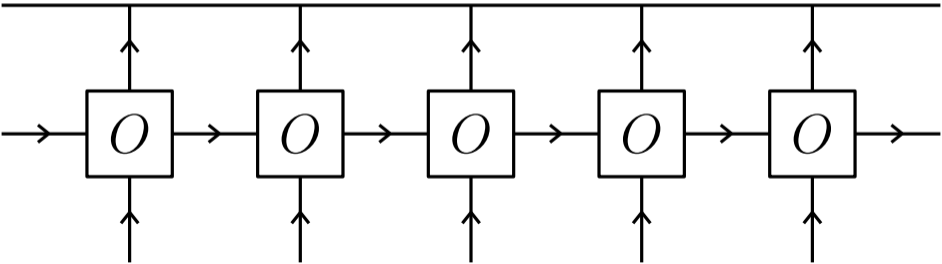

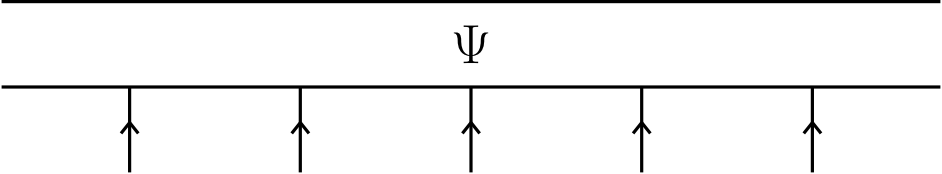

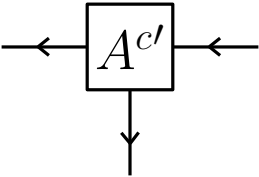

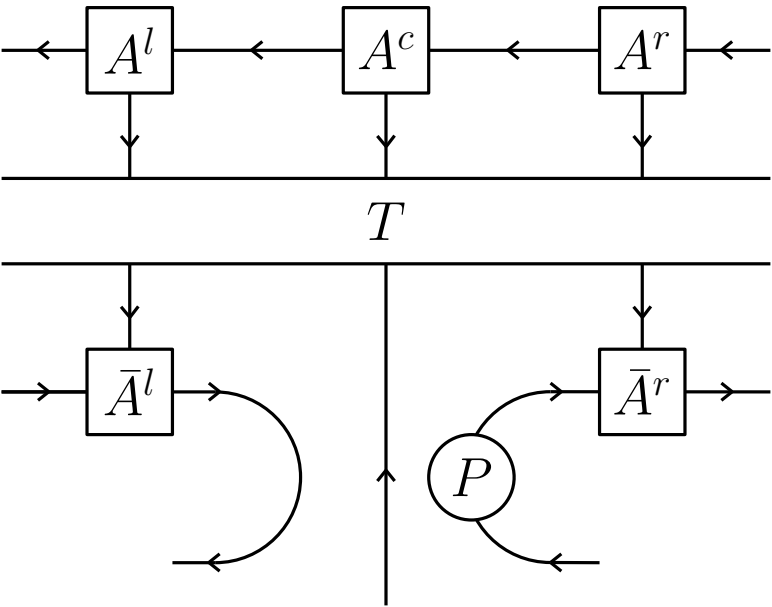

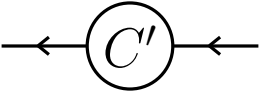

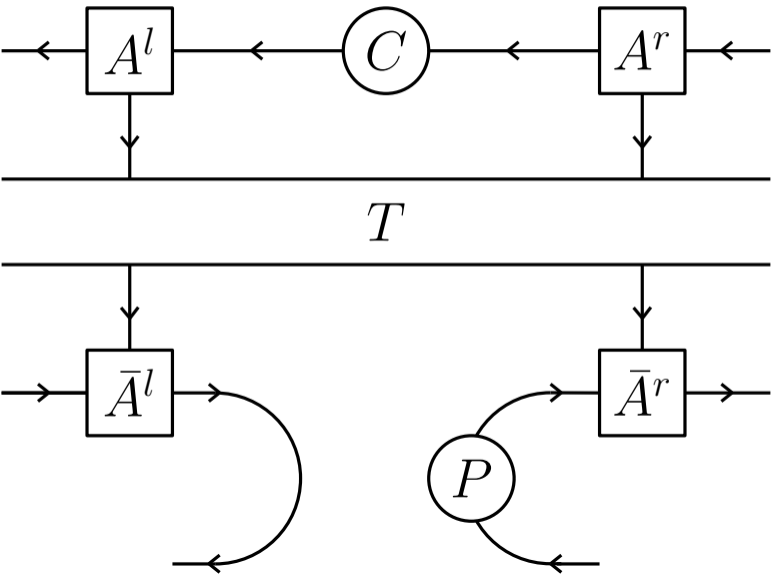

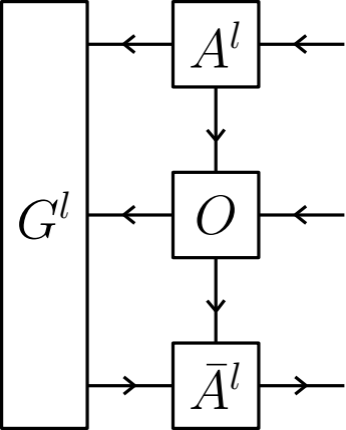

$G^l$

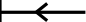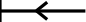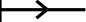

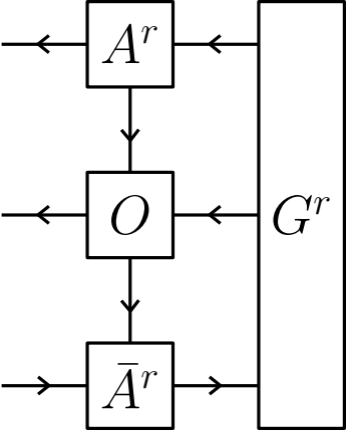

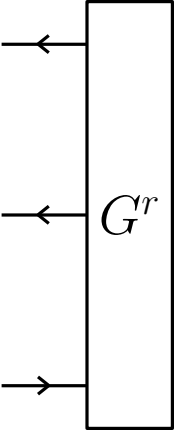

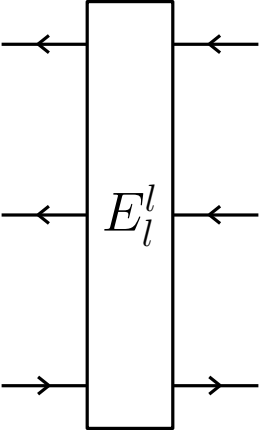

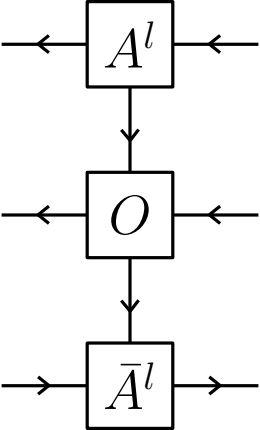

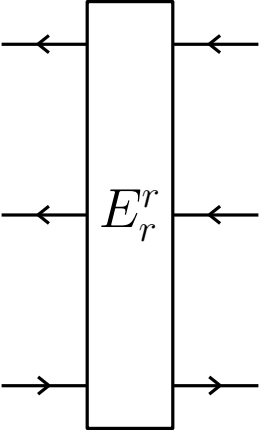

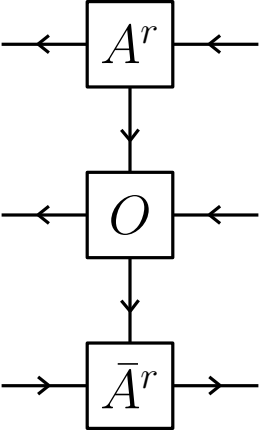

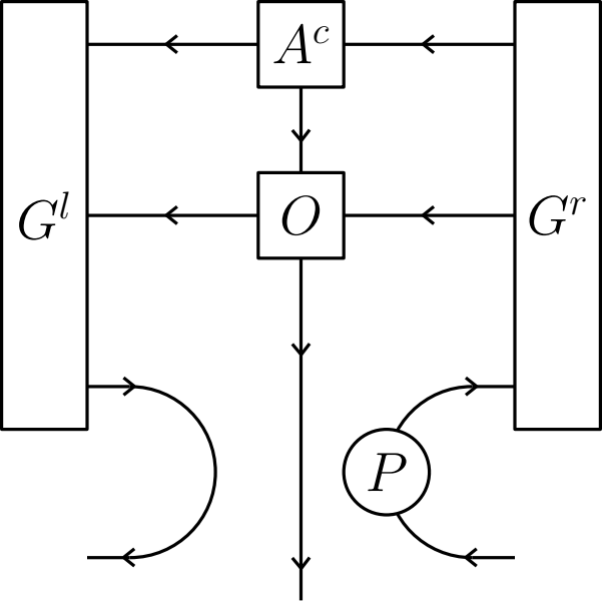

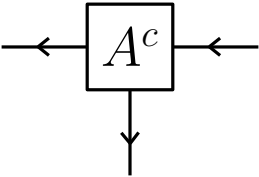

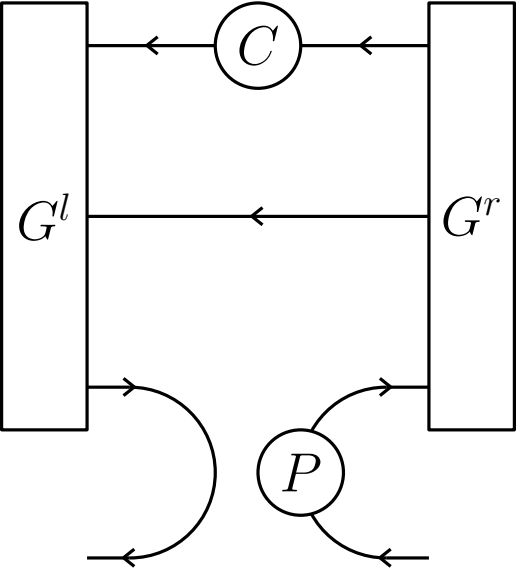

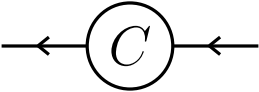

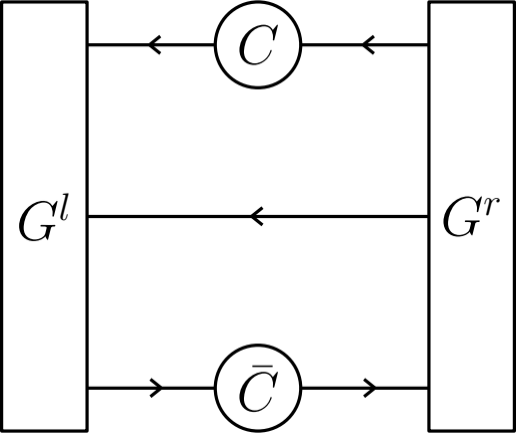

$\beta$

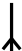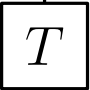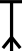

$\alpha$

$\alpha$

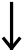

$\bar{T}$

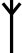

$\beta$

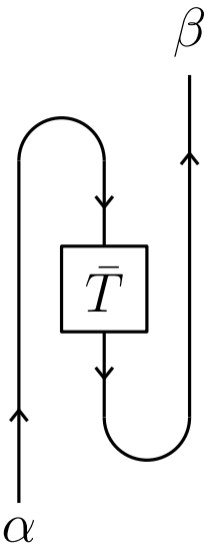

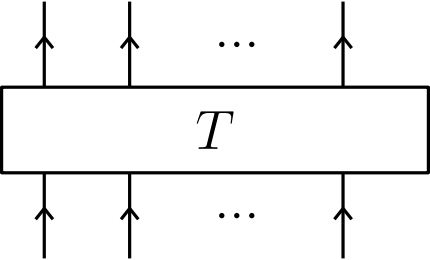

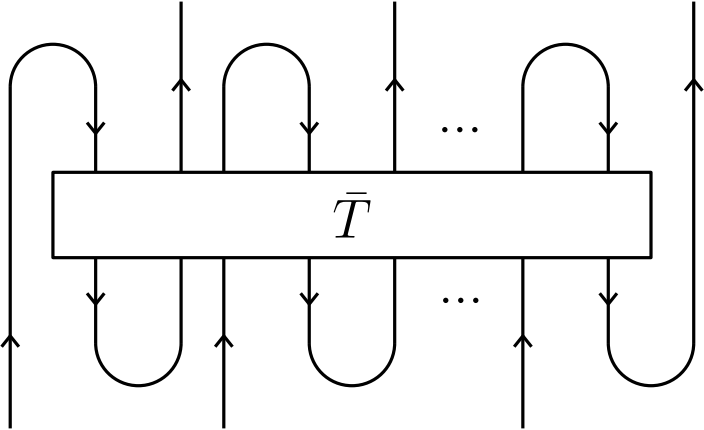

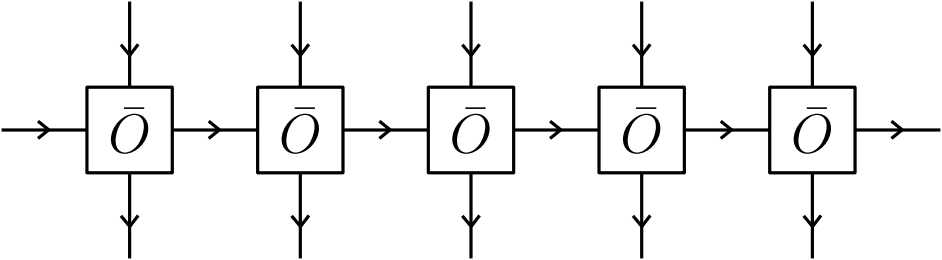

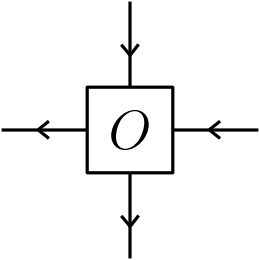

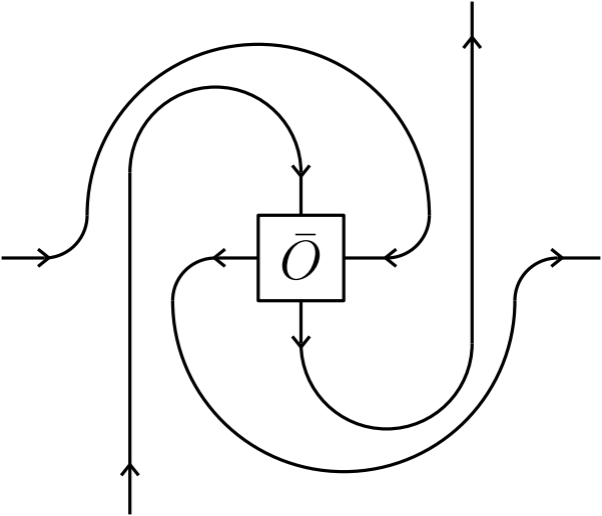

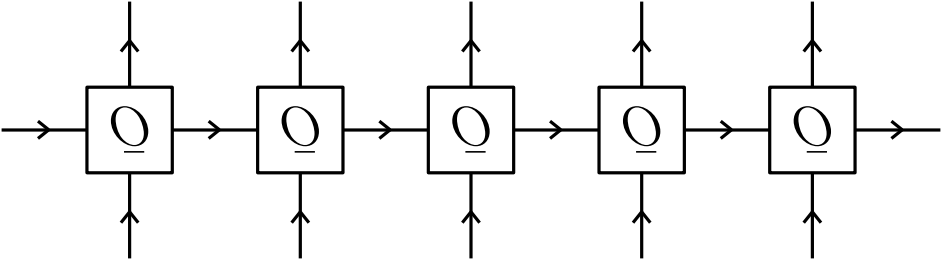

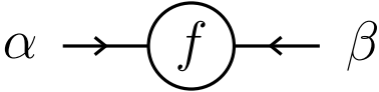

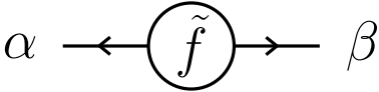

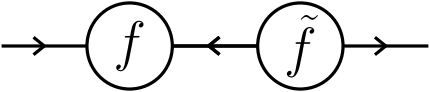

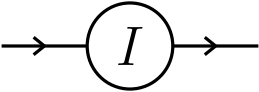

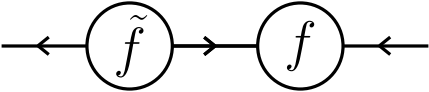

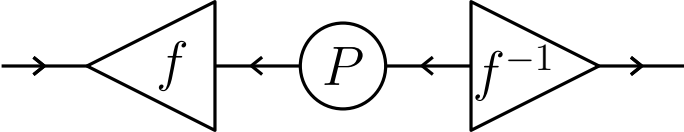

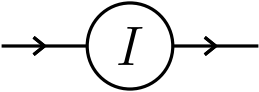

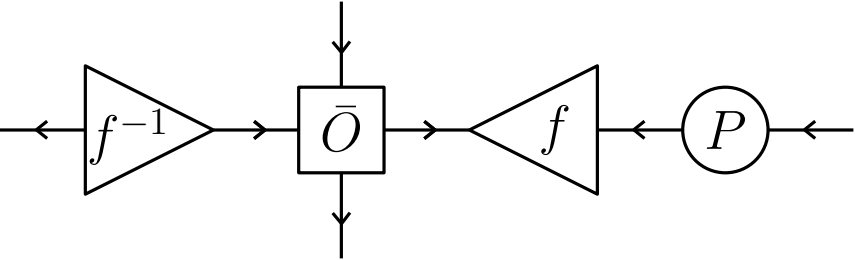

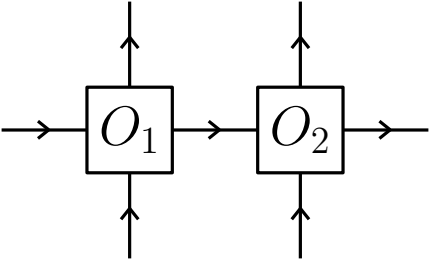

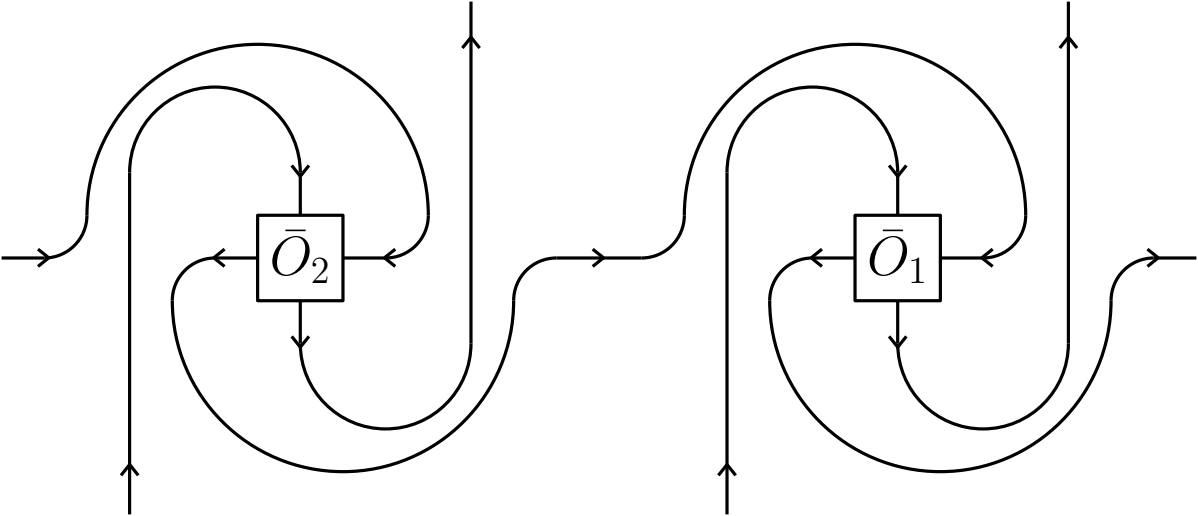

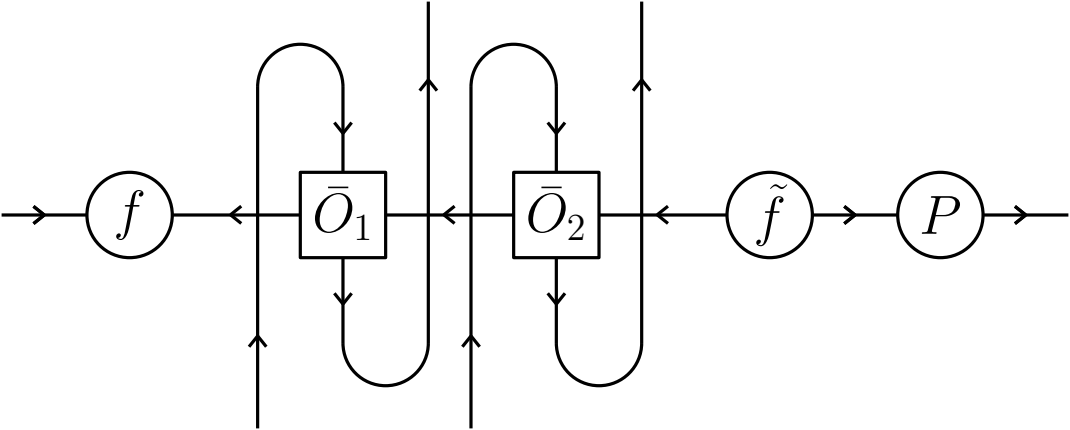

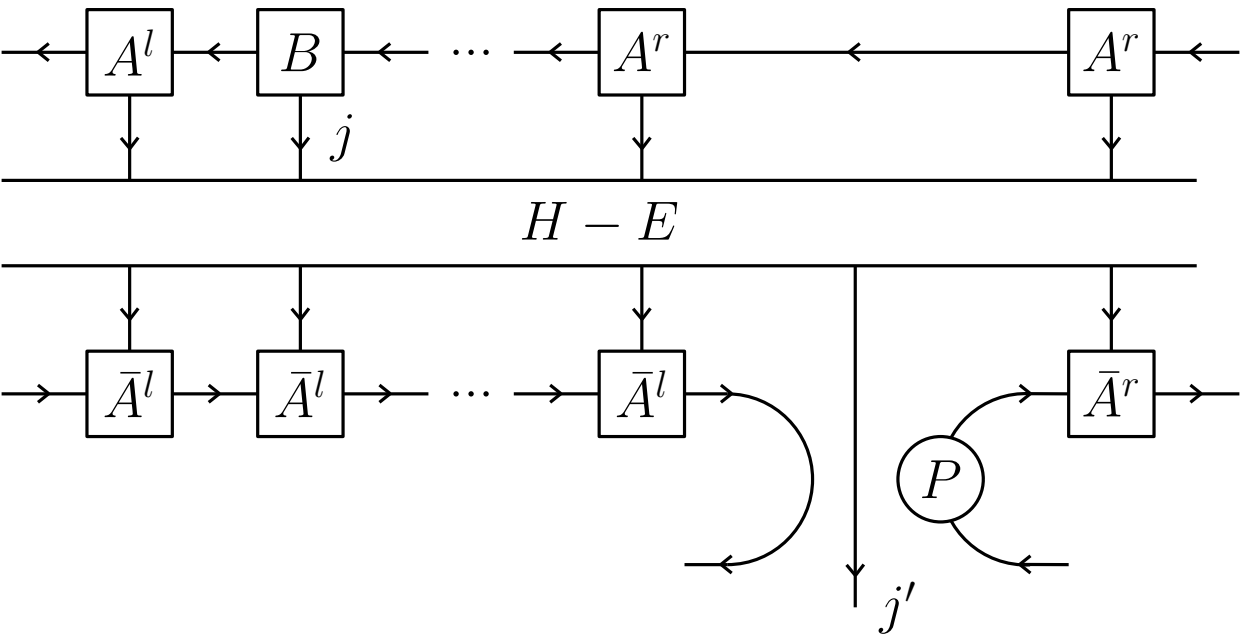

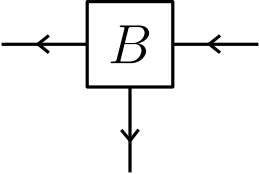

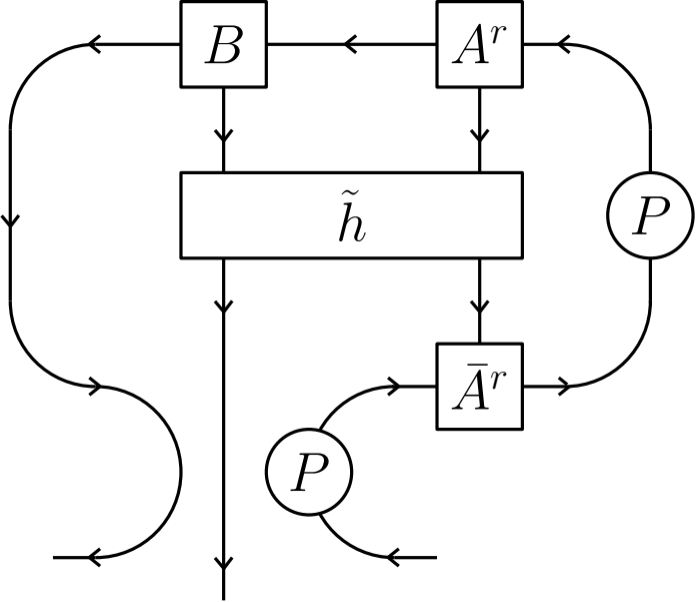

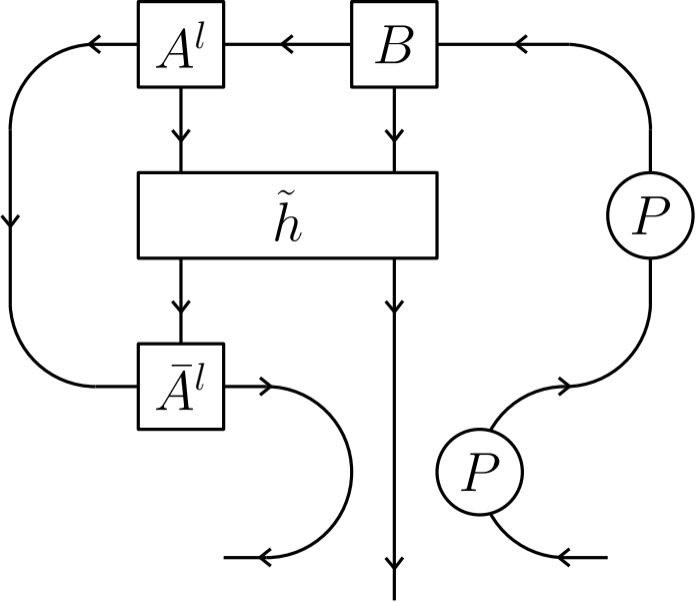

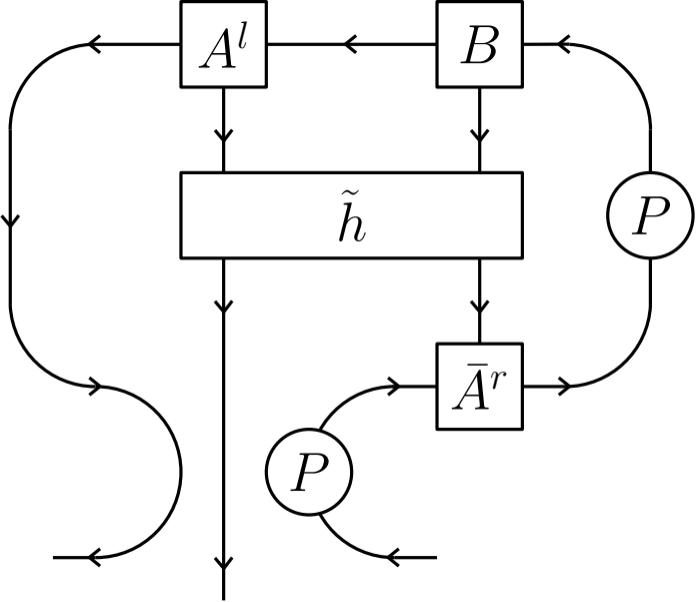

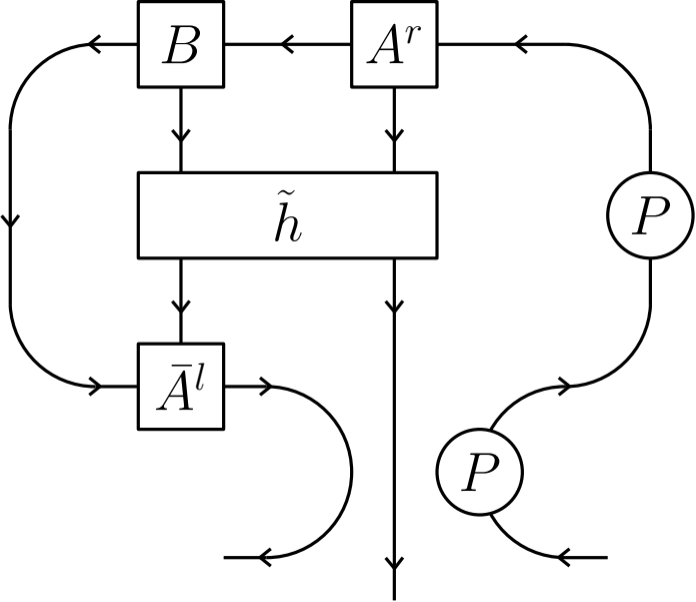

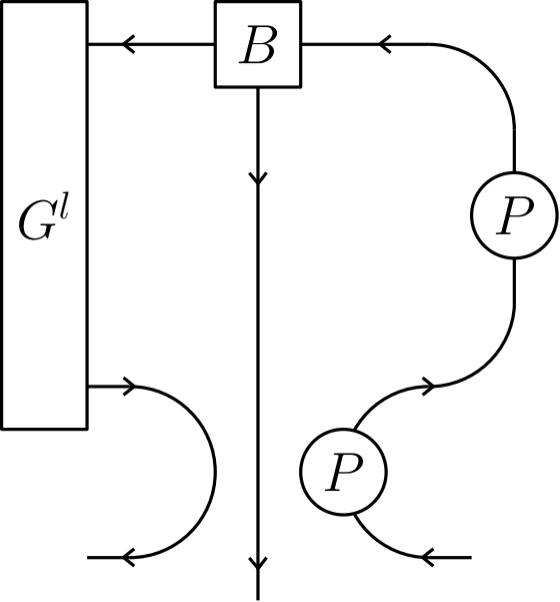

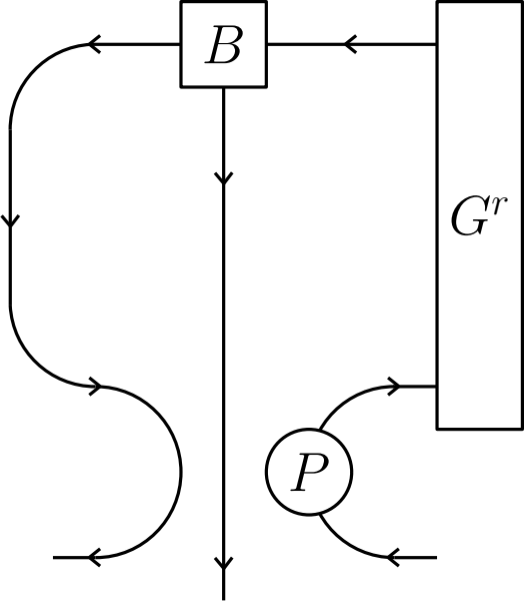

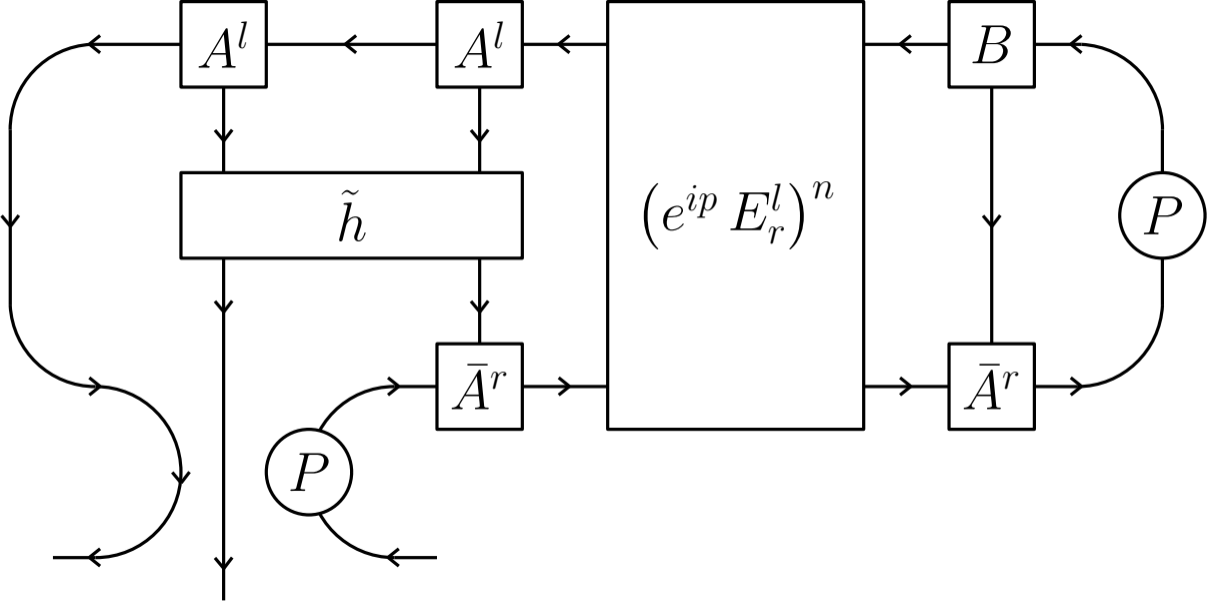

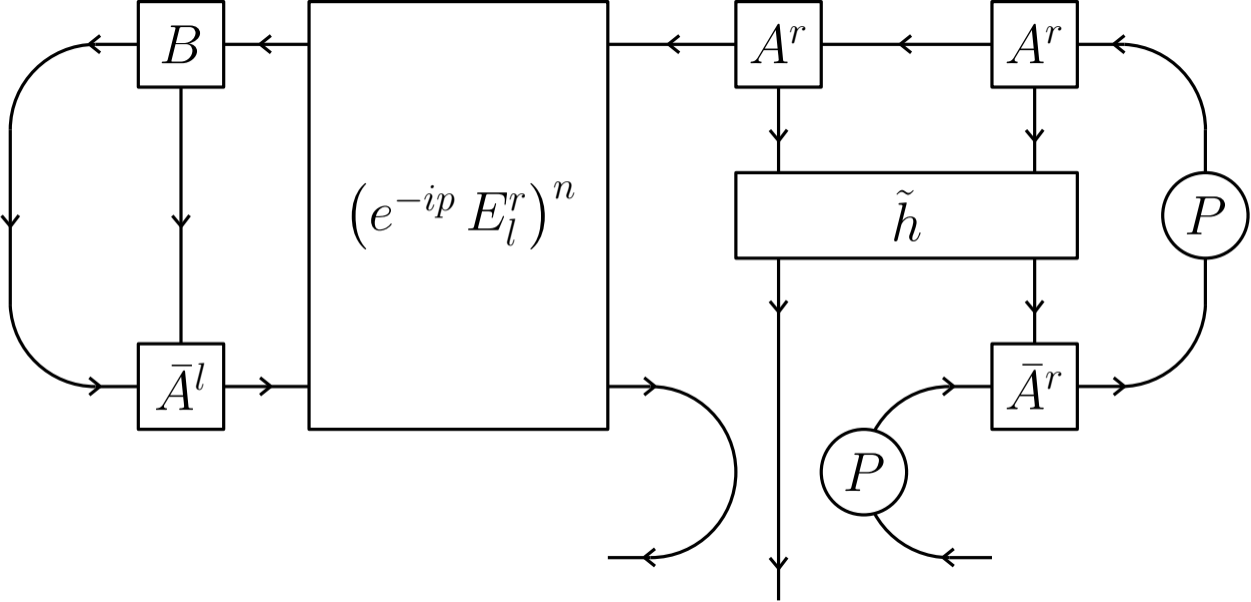

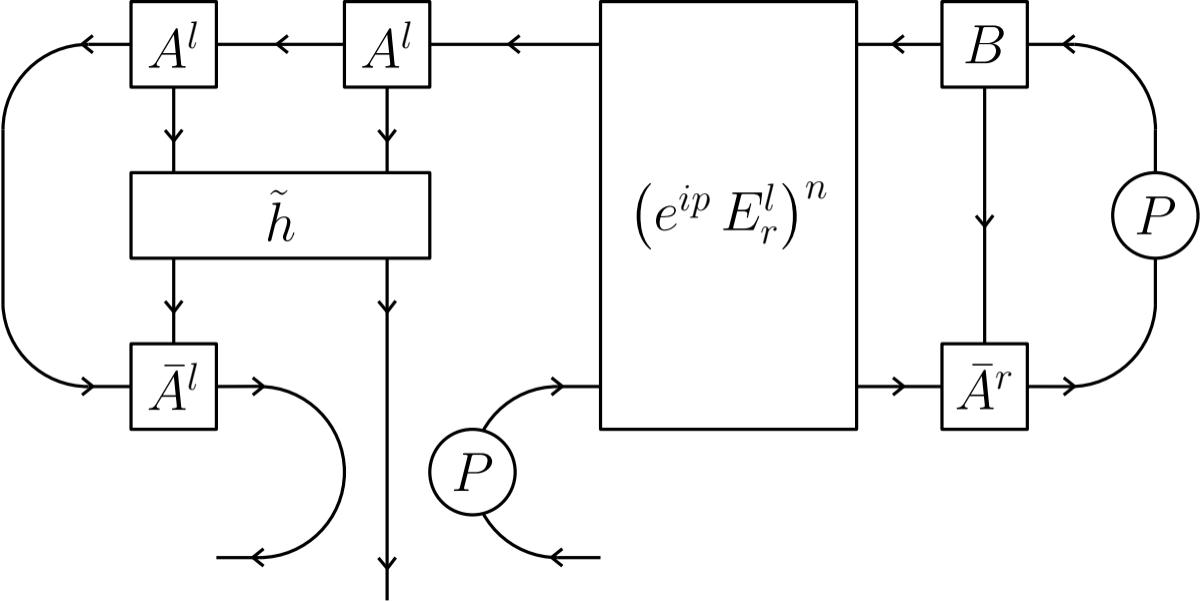

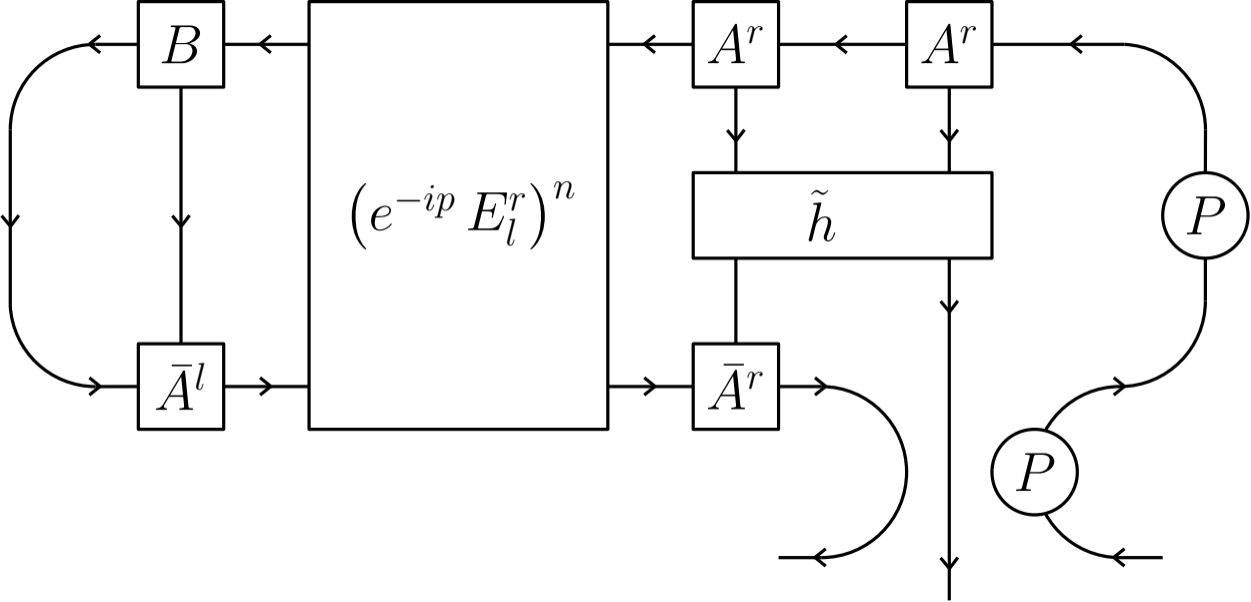

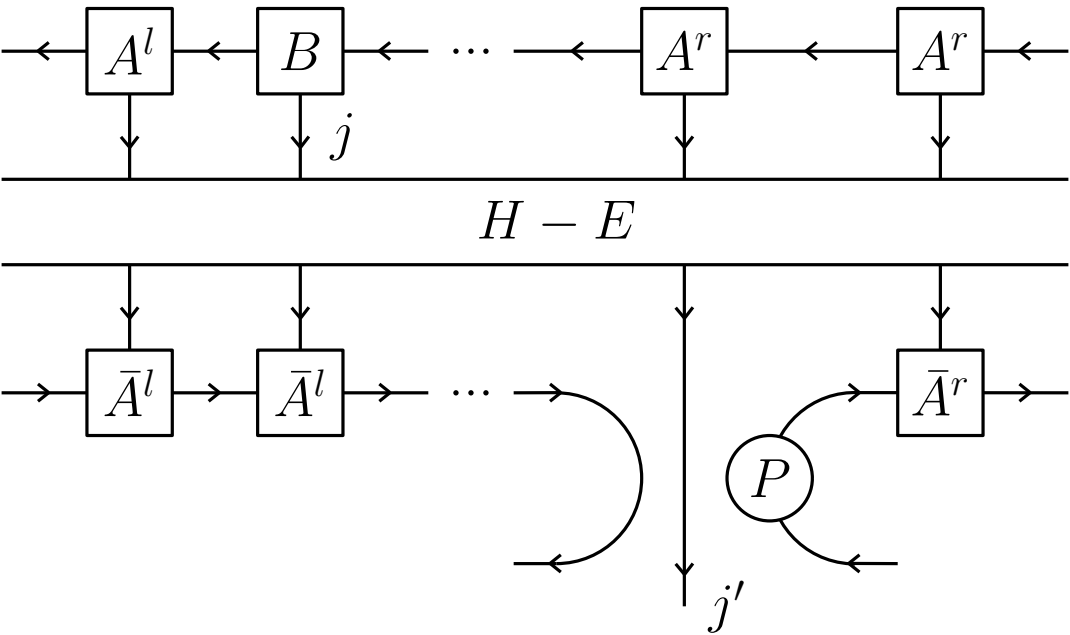

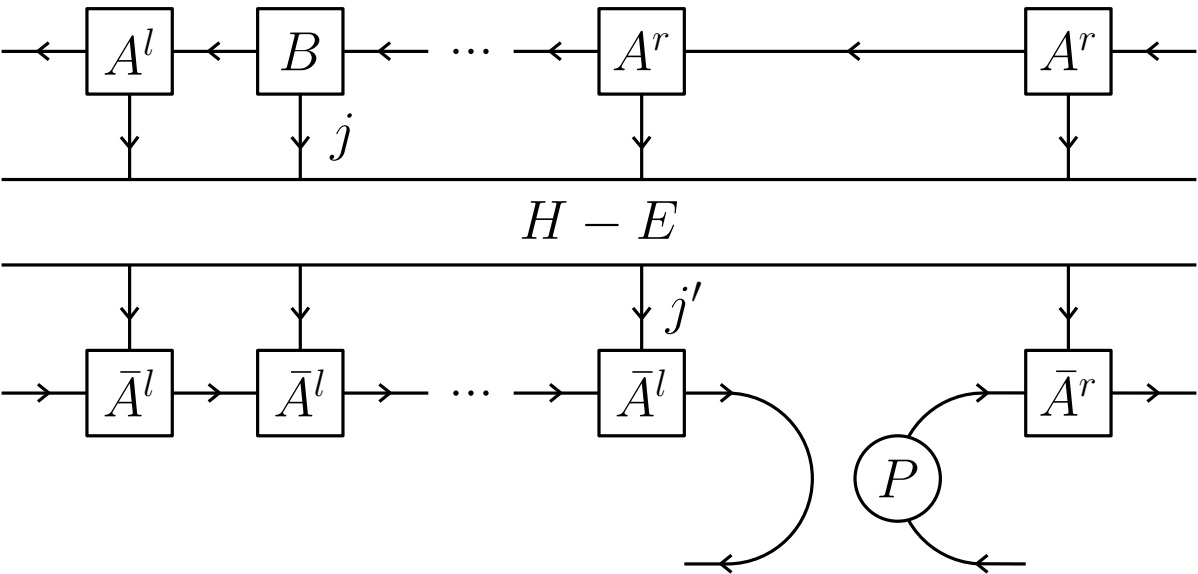

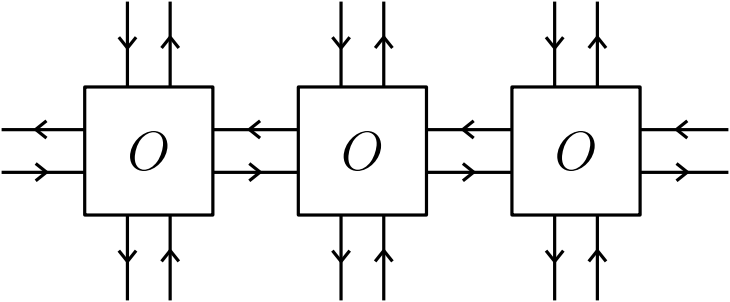

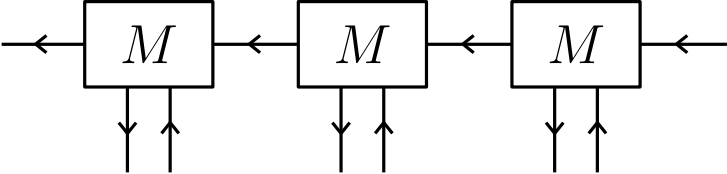

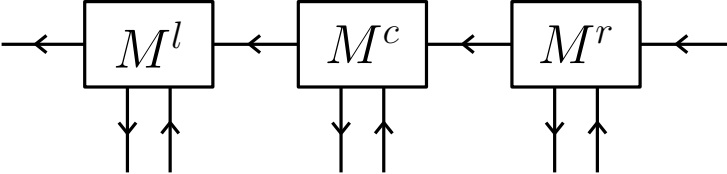

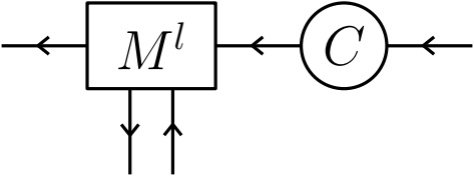

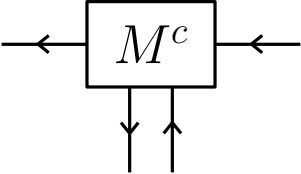

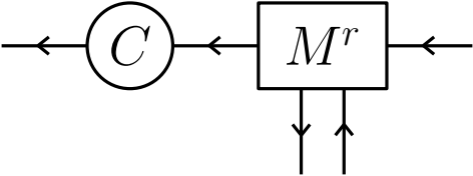

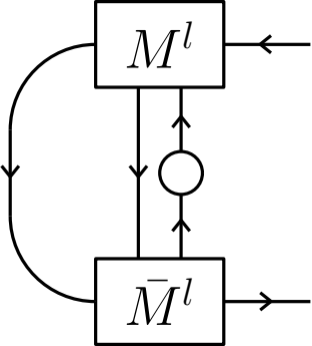

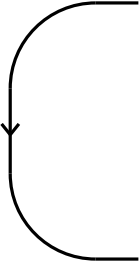

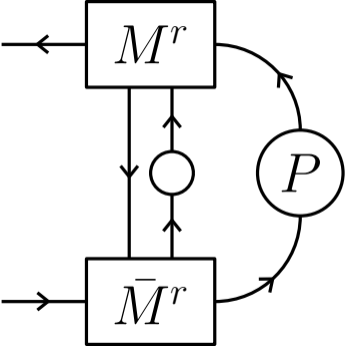

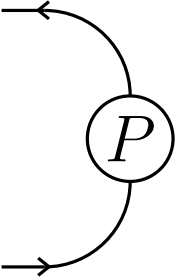

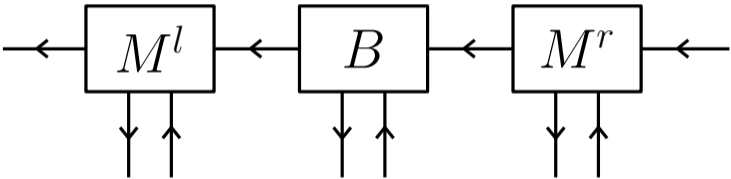

$j$

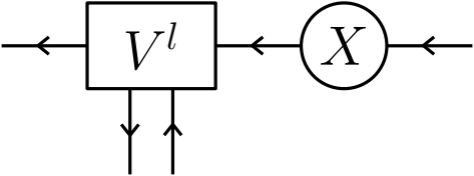

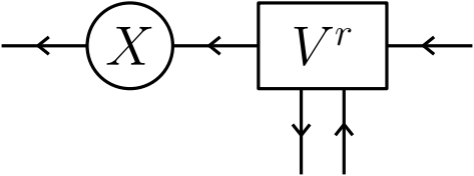

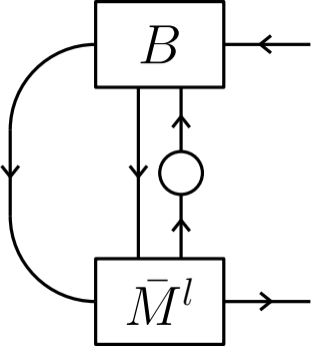

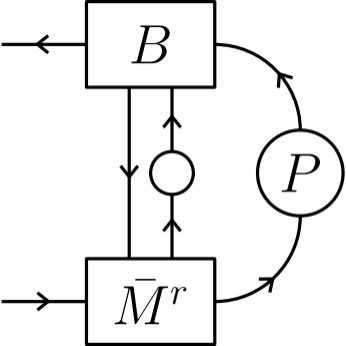

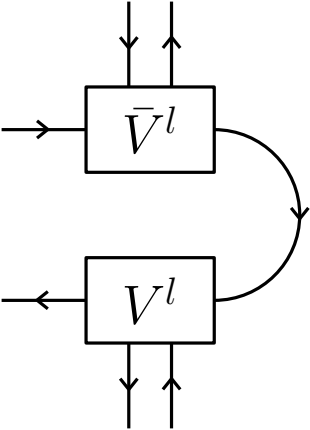

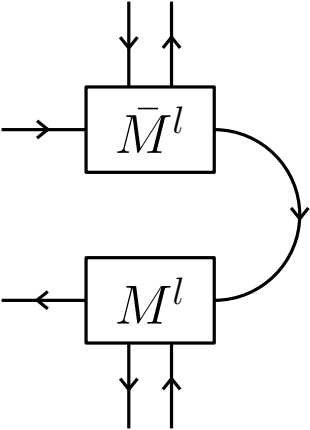

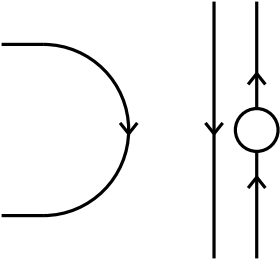

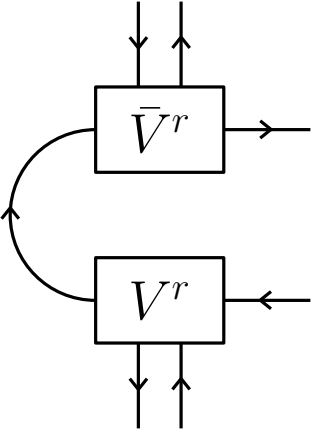

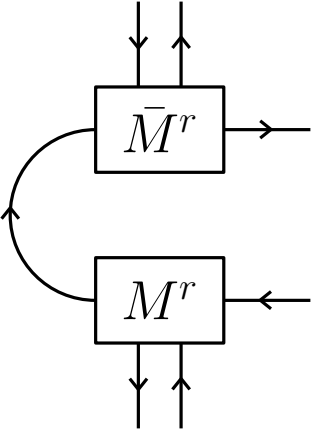

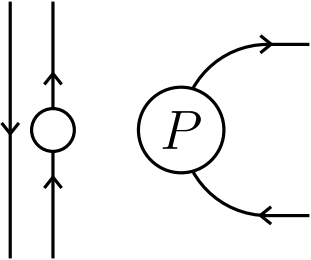

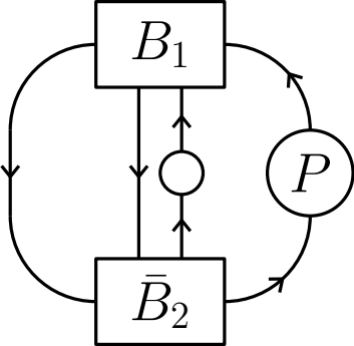

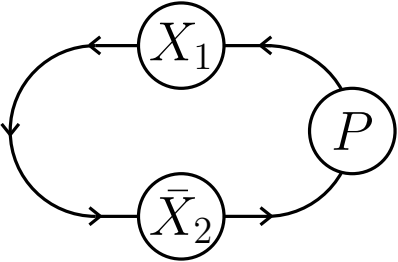

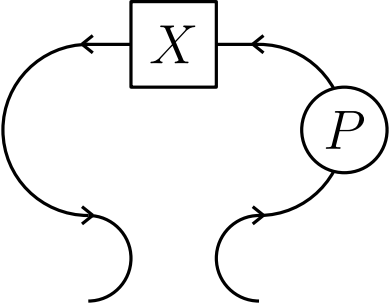

$\chi$

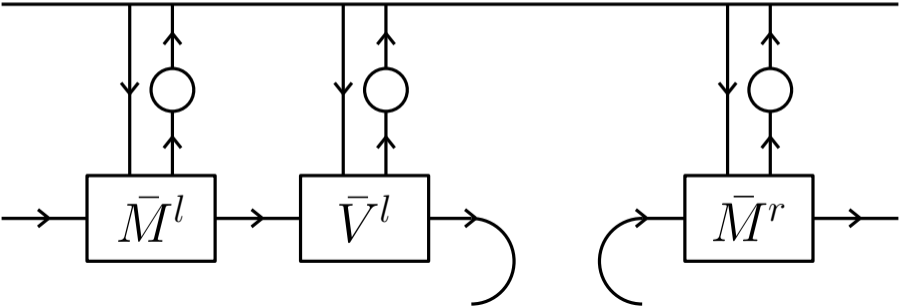

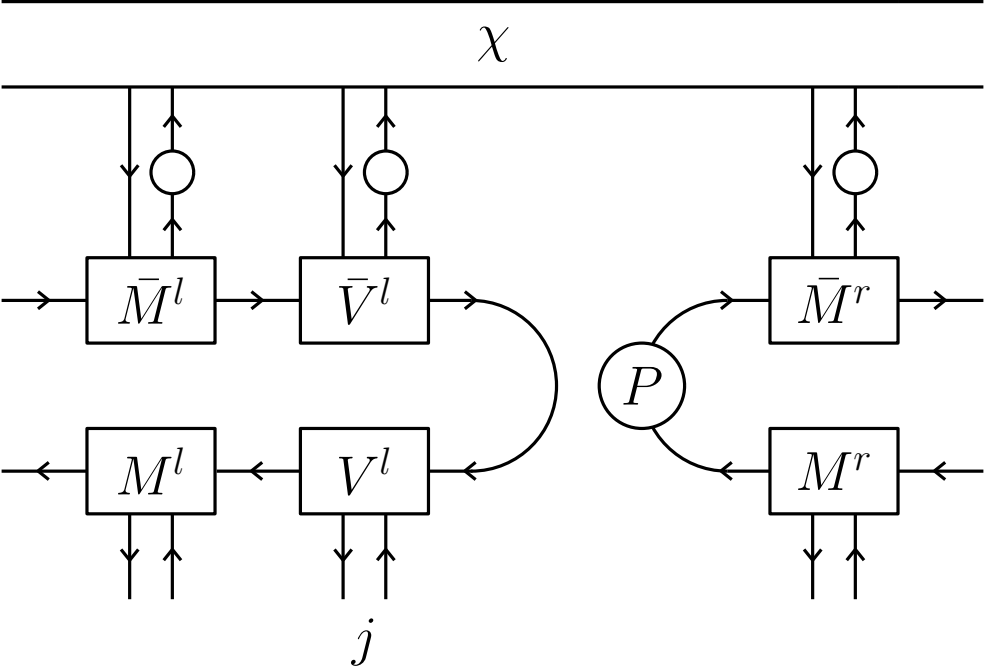

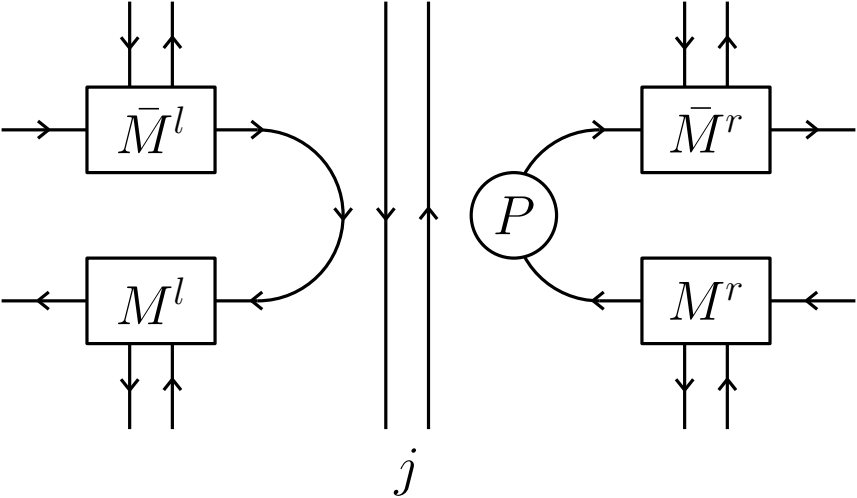

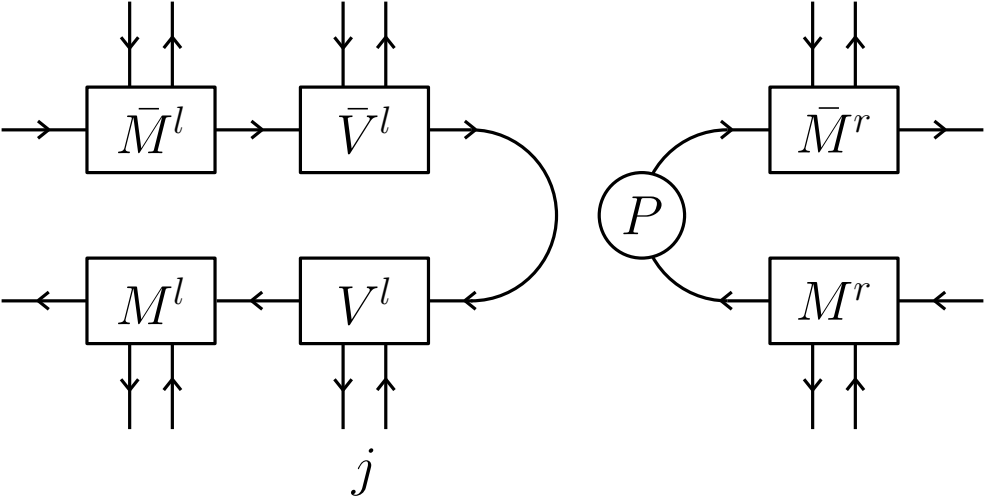

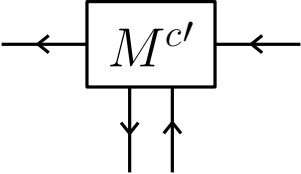

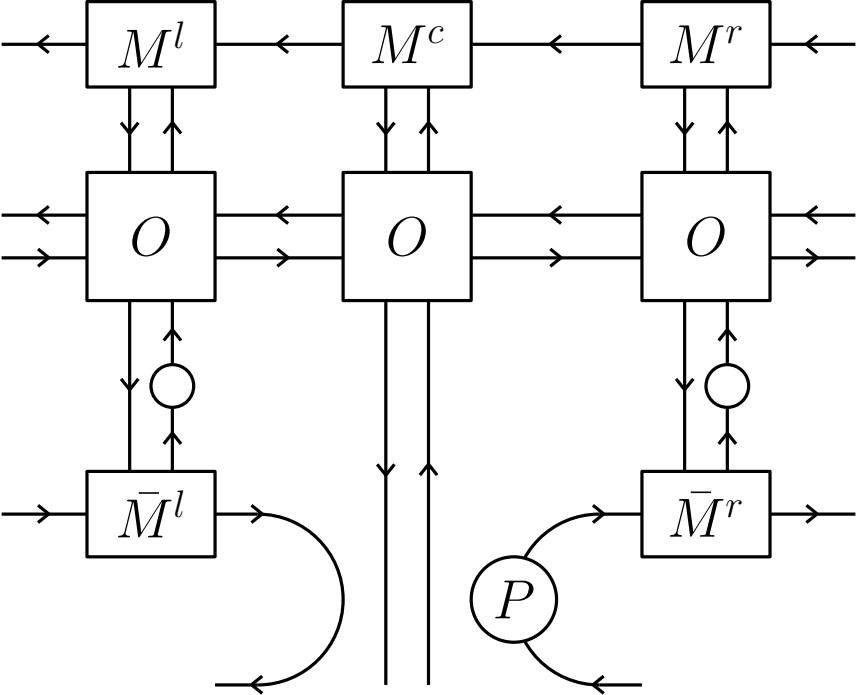

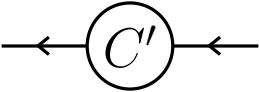

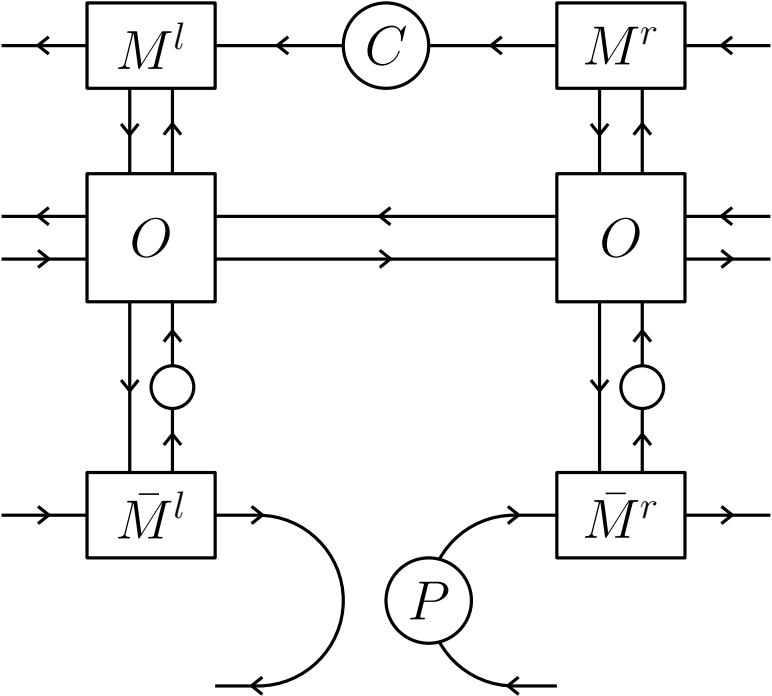

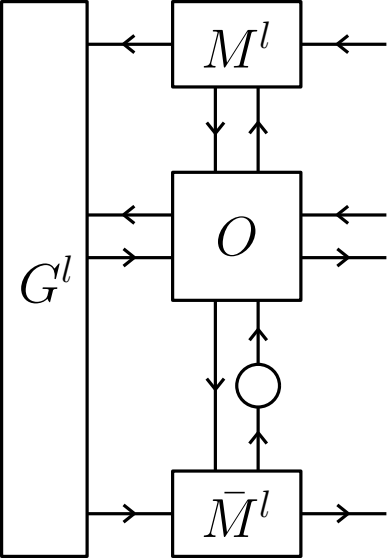

$G^l$

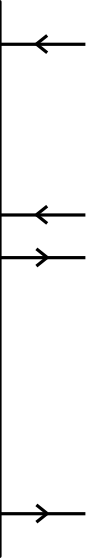

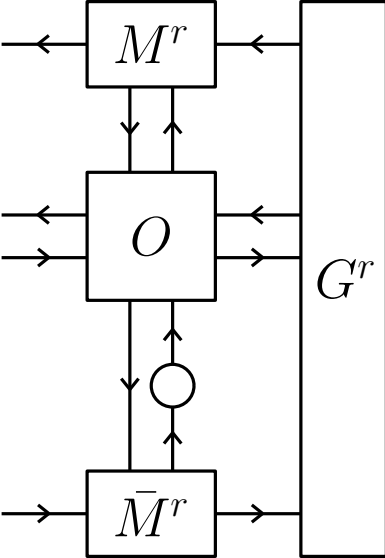

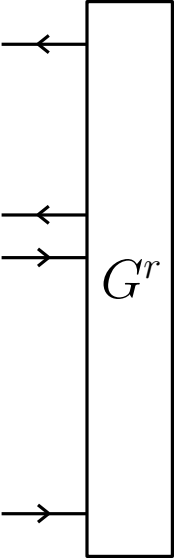

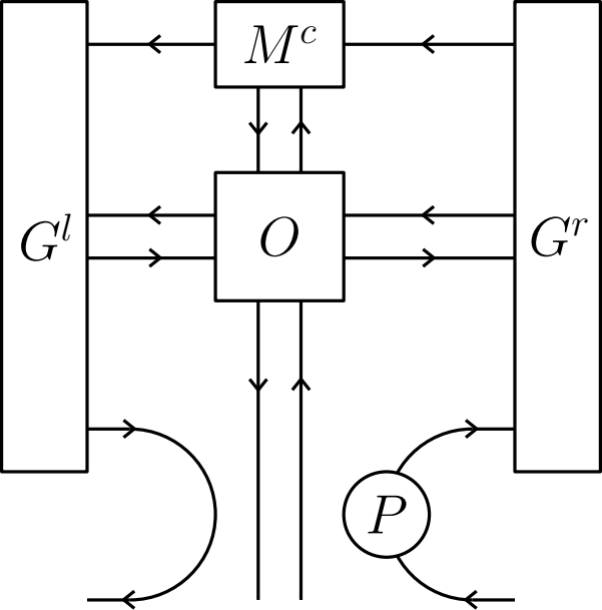

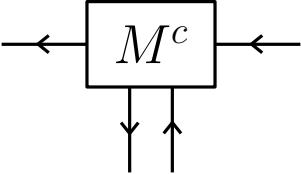

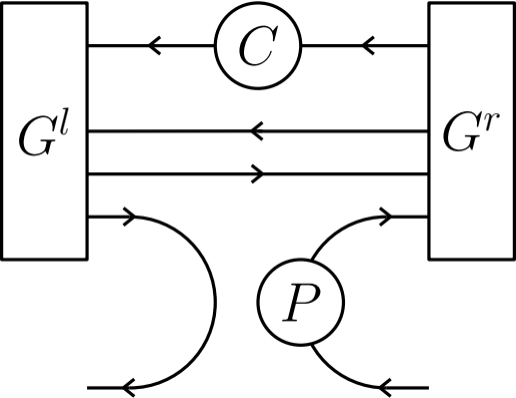

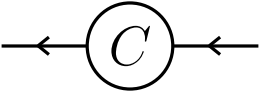

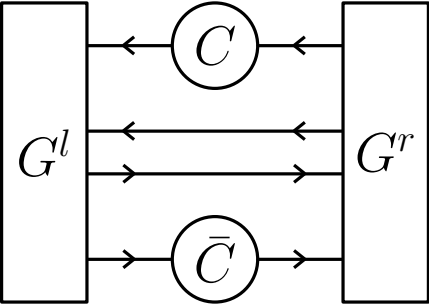

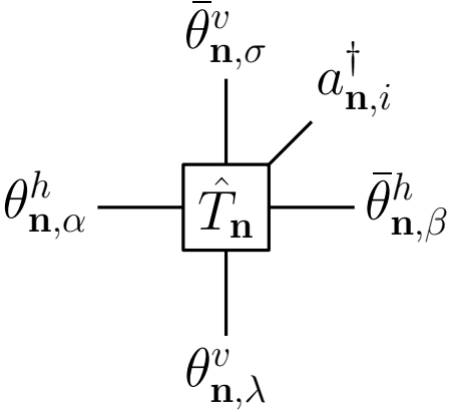

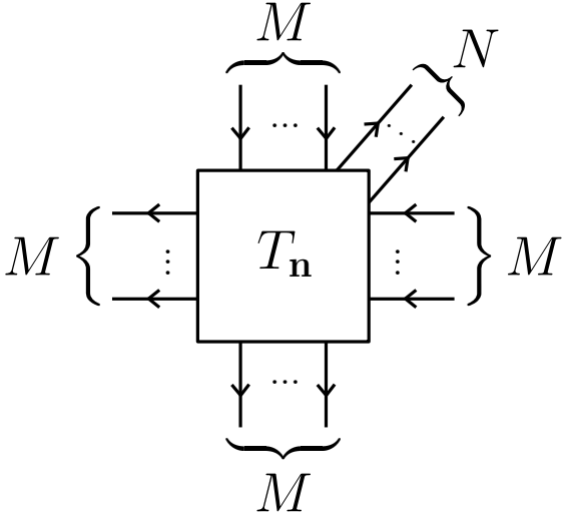

Supplement: Supplementary file 1 [file appendix.pdf]
